# Supplementary material for: Learning curves for the multi-class teacher-student perceptron
Source: arXiv:2203.12094 source file (2022-03-22)
Supplement: Supplementary file 1 [file update_functions.tex]

\section{Definitions of the update functions}
\subsection{Prior terms}
\begin{align}
       {\cal Z}_{0} ( \bm{\gamma}, \bm{\Lambda} ) &= \int_{\mathbb{R}^K} \dde \bm{w}  P_{0} ( \bm{w} )  e^{- \frac{1}{2} \bm{w}^{\top} \bm{\Lambda} \bm{w} + \bm{\gamma}^{\top} \bm{w}   } \;,
\end{align}
\begin{equation}
\bm{f}_{0} ( \bm{\gamma}, \bm{\Lambda}  ) \equiv \partial_{\bm{\gamma}} \log  {\cal Z}_{0} ( \bm{\gamma}, \bm{\Lambda} ).
\end{equation}
In the following we want to consider the ERM $\ell_2-$regularization prior, with the mapping defined in Appendix \ref{appendix:mapping}. This means that 
\begin{align}
P_0(\bm{w}) = \frac{1}{(2 \pi)^{K/2} \sqrt{\det(\bm{C}/(\beta \lambda)}}\exp\left(-\frac{\beta\lambda}{2}  \bm{w}^\top \bm{C}^{-1}\bm{w}\right),
\end{align}
where $C$ is the prior covariance in the reduced setting, i.e. $C:= [2,1; 1,2]$.
Let $\beta\bm{\gamma}=\beta\bm{\hat q}^{1/2}\bm\xi$ and $\beta\bm{\Lambda}=\beta\bm{\hat V}$. Once we have introduced the rescaling {\color{red} explain somewhere}, we obtain
\begin{align}
{\cal Z}_{0} ( \bm{\gamma}, \bm{\Lambda} ) &= \int_{\mathbb{R}^K}\dde\bm{w}\, \frac{e^{-\frac{\beta}{2} \bm{w}^{\top}(\lambda \bm{C^{-1}}+ \bm{\Lambda}) \bm{w} + \beta\bm{\gamma}^\top \bm{w}   } }{(2 \pi)^{K/2} \sqrt{\det (\bm{C}/\beta \lambda)}} =\frac{1}{\sqrt{\det(\bm{C}/\beta \lambda) \det(\beta\lambda\bm{C^{-1}}+\beta\bm{\Lambda})}}\exp\left(\frac{\beta}{2}\bm{\gamma}^\top (\lambda\bm{C^{-1}}+\bm{\Lambda})^{-1}\bm{\gamma}\right)\;,\\
\bm{f}_{0} ( \bm{\gamma}, \bm{\Lambda}  )&=\beta\,(\lambda \bm{C^{-1}}+\bm{\Lambda})^{-1} \bm{\gamma},\\
\partial_{\bm{\gamma}}\bm{f}_{0} ( \bm{\gamma}, \bm{\Lambda}  )&=\beta (\lambda\bm{C^{-1} }+\Lambda)^{-1}.
\end{align}
{\color{red} explain again consistency with rescaling of overlaps}
Similarly, we can compute the Gaussian teacher prior terms with the reduction:
\begin{align}
       {\cal Z}^*_{0} ( \bm{\gamma}, \bm{\Lambda} ) &= \int_{\mathbb{R}^K} \frac{d \bm{w}}{\sqrt{(2\pi)^K\det(\bm{C})}}    e^{- \frac{1}{2} \bm{w}^{\top} (\bm{C^{-1}}+\bm{\Lambda}) \bm{w} + \bm{\gamma}^{\top} \bm{w}   } =\frac{1}{\sqrt{\det(\bm{C})\det(\bm{C^{-1}}+\bm{\Lambda})}}\exp\left(\frac{1}{2}\bm{\gamma}^\top (\bm{C^{-1}}+\bm{\Lambda})^{-1}\bm{\gamma}\right)\;,\\
\bm{f}^*_{0} ( \bm{\gamma}, \bm{\Lambda}  ) &= \partial_{\bm{\gamma}} \log  {\cal Z}^*_{0} ( \bm{\gamma}, \bm{\Lambda} ) = (\bm{C^{-1}}+\bm{\Lambda})^{-1}\bm{\gamma} \;,\\
\partial_{\bm \gamma}\bm{f}^*_{0} ( \bm{\gamma}, \bm{\Lambda}  ) &=(\bm{C^{-1}}+\bm{\Lambda})^{-1}.
\end{align}
Recall, the saddle point equations for parameters $(\bm{m},\bm{q},\bm{V})$ are the following (Theorem~\ref{thm:ERM_main}):
\begin{align}
    \bm{m}&=\mathbb{E}_{\bm \xi}\left[\mathcal{Z}^*_0 \, \times  \bm{f}^*_0(\bm{\hat m}\bm{\hat q}^{-1/2}\bm{\xi},\bm{\hat m}^T\bm{\hat q}^{-1}\bm{\hat m})\,\bm{f}_0(\bm{\hat q}^{1/2}\bm{\xi},\bm{\hat V})^\top\right],\\
    \bm{q}&=\mathbb{E}_{\bm \xi}\left[\mathcal{Z}^*_0(\bm{\hat m}\bm{\hat q}^{-1/2}\bm{\xi},\bm{\hat m}^T\bm{\hat q}^{-1}\bm{\hat m})\,\bm{f}_0(\bm{\hat q}^{1/2}\bm{\xi},\bm{\hat V})\bm{f}_0(\bm{\hat q}^{1/2}\bm{\xi},\bm{\hat V})^\top\right],\\
    \bm{V}&=\mathbb{E}_{\bm \xi}\left[\mathcal{Z}^*_0(\bm{\hat m}\bm{\hat q}^{-1/2}\bm{\xi},\bm{\hat m}^T\bm{\hat q}^{-1}\bm{\hat m})\partial_{\bm{\gamma}}\bm{f}_0(\bm{\hat q}^{1/2}\bm{\xi},\bm{\hat V})\right].
\end{align}
Thus, substituting the expressions above we find:
% $\bm{C}:=[2,1;1,2]$,
\begin{align}
\bm{m}&=\frac{\beta}{\sqrt{\det(\bm{C})\det \bm{C}^{-1}+\bm{\hat m}\bm{ \hat q}^{-1}\bm{\hat m})}\sqrt{\det(\bm{I}-\bm{\hat q}^{-1/2}\bm{\hat m}(\bm{C}^{-1}+\bm{\hat m}\bm{\hat q}^{-1}\bm{\hat m})^{-1}\bm{\hat m}\bm{\hat q}^{-1/2})}}\\
&\times( \bm{C}^{-1} +\bm{\hat m}\bm{\hat q}^{-1}\bm{\hat m})^{-1} \bm{\hat m} \bm{\hat q}^{-1/2}\left(\bm{I}-\bm{\hat q}^{-1/2}\bm{\hat m}(\bm{C}^{-1}+\bm{\hat m}\bm{\hat q}^{-1}\bm{\hat m})^{-1} \bm{\hat m} \bm{\hat q}^{-1/2}\right)^{-1}\bm{\hat q^{1/2}}(\lambda \bm{C}^{-1}+\bm{\hat V})^{-1}\;,\\
\bm{q}&=\frac{\beta^2}{\sqrt{\det(\bm{C})\det(\bm{C}^{-1}+\bm{\hat m}\bm{ \hat q}^{-1}\bm{\hat m})}\sqrt{\det(\bm{I}-\bm{\hat q}^{-1/2}\bm{\hat m}(\bm{C}^{-1}+\bm{\hat m}\bm{\hat q}^{-1}\bm{\hat m})^{-1}\bm{\hat m}\bm{\hat q}^{-1/2})}}\\
&\times (\lambda \bm{C}^{-1}+\bm{\hat V})^{-1} \bm{\hat q}^{1/2}\left(\bm{I}-\bm{\hat q}^{-1/2}\bm{\hat m}(\bm{C}^{-1}+\bm{\hat m}\bm{\hat q}^{-1}\bm{\hat m})^{-1} \bm{\hat m} \bm{\hat q}^{-1/2}\right)^{-1}\bm{\hat q}^{1/2}(\lambda \bm{C}^{-1}+\bm{\hat V})^{-1}
\;,\\
\bm{V}&=\frac{\beta(\lambda \bm{C}^{-1}+\bm{\hat V})^{-1}}{\sqrt{ \det(\bm{C})\det(\bm{C}^{-1}+\bm{\hat m}\bm{ \hat q}^{-1}\bm{\hat m})}\sqrt{\det(\bm{I}-\bm{\hat q}^{-1/2}\bm{\hat m}(\bm{C}^{-1}+\bm{\hat m}\bm{\hat q}^{-1}\bm{\hat m})^{-1}\bm{\hat m}\bm{\hat q}^{-1/2})}}.
\end{align}
\subsection{Channel terms}
